# Supplementary material for: AutoFish: Dataset and Benchmark for Fine-grained Analysis of Fish
Source: arXiv:2501.03767 source file (2025-01-07)
Supplement: Supplementary file 1 [file supplementary.tex]

Don't know if we are gonna include this section.
However, so far it contains some figures and result tables regarding the balanced vs imbalanced dataset splits.
This is followed by the class-granularity stuff, where we show that the classification works really well independent on whether we only look for "fish vs no fish" or when including all six species.

\begin{figure*}
    \centering

    \begin{subfigure}{\textwidth}
        \centering
        \includegraphics[width=0.8\linewidth]{figures/splits/balanced.png}
        \caption{The balanced split}
        \label{fig:subfiga}
    \end{subfigure}

    \vspace{\baselineskip} % Vertical space between subfigures

    \begin{subfigure}{\textwidth}
        \centering
        \includegraphics[width=0.8\linewidth]{figures/splits/unbalanced_A.png}
        \caption{The imbalanced split A}
        \label{fig:subfigb}
    \end{subfigure}

    \vspace{\baselineskip} % Vertical space between subfigures

    \begin{subfigure}{\textwidth}
        \centering
        \includegraphics[width=0.8\linewidth]{figures/splits/unbalanced_B.png}
        \caption{The imabalaned split B}
        \label{fig:subfigc}
    \end{subfigure}

    \caption{The species distribution of the train and test groups of the three proposed dataset splits.}
    \label{fig:dataset_splits}
\end{figure*}

\begin{table}
    \centering
    \caption{Split-specific test groups.}
    \label{tab:dataset_splits}
    \begin{tabular*}{\linewidth}{@{\extracolsep{\fill}} cc}
        \toprule
        \textbf{Split} & \textbf{Test Groups} \\
        \midrule
        \rowcolor[HTML]{EFEFEF}Balanced & 10, 14, 20, 21, 22 \\
        Imbalanced A & 2, 15, 16, 19, 25 \\
        \rowcolor[HTML]{EFEFEF}Imbalanced B  & 1, 3, 4, 8, 13 \\
        \bottomrule
    \end{tabular*}
\end{table}

\subsubsection{Imbalanced training}
The outcome of comparing training on balanced versus imbalanced splits can be seen in Table~\ref{tab:balanced_imbalaned_results}. The results shows that optimal performance is achieved on the balanced split for both backbone architectures along with a comparable overall performance when tested on imbalanced splits. Despite the lower overall performance on imbalanced splits compared to the balanced split, the disproportionate class distribution between the training and testing splits does not seem to detrimentally affect class-specific performance.

In imbalanced split A, where the number of cod instances used in training is considerably lower than in testing, the performance remains comparable to that observed in the balanced split. A similar pattern is observed for whiting and hake in imbalanced split B. The most notable decline in performance occurs in the \textit{other} class when transitioning from balanced to imbalanced splits.

\begin{table*}
    \centering
   \caption{Performance comparison between training on the balanced and imbalanced splits.}
    \label{tab:balanced_imbalaned_results}
    \begin{tabular*}{\linewidth}{@{\extracolsep{\fill}} lcccccccc} 
    \toprule
        \textbf{Model} & \textbf{Split} & \textbf{AP} & \textbf{Whiting} & \textbf{Cod} & \textbf{Haddock} & \textbf{Hake} & \textbf{Horse mackerel} & \textbf{Other} \\ \midrule
        R-50 & balanced & 88.37 & 90.37 & 86.96 & 88.49 & 86.49 & 87.67 & 90.24 \\
        Swin-B & balanced & \textbf{89.47} & \textbf{91.26} & \textbf{88.23} & \textbf{90.00} & \textbf{87.44} & \textbf{88.51} & \textbf{91.38} \\ \midrule
        R-50 & imbalanced A & \textbf{85.84} & \textbf{87.65} & \textbf{86.64} & \textbf{87.79} & 83.00 & 88.76 & \textbf{81.23} \\ 
        Swin-B & imbalanced A & 85.72 & 87.25 & 86.26 & 87.61 & \textbf{84.97} & \textbf{89.43} & 78.81 \\ \midrule 
        R-50 & imbalanced B & 86.29 & 90.24 & \textbf{88.96} & 90.00 & \textbf{87.91} & \textbf{84.57} & 76.05 \\ 
        Swin-B & imbalanced B & \textbf{86.36} & \textbf{90.40} & 88.84 & \textbf{90.81} & 87.29 & 80.81 & \textbf{80.03} \\ \bottomrule
    \end{tabular*}
\end{table*}

\iffalse{
    \begin{figure}
        \centering
        \includegraphics[width=\linewidth]{figures/experiments/balanced_vs_unbalanced.pdf}
        \caption{Your Figure Caption Here}
        \label{fig:balanced_unbalaced_label_configurations}
    \end{figure}
        
    \begin{figure}[h]
        \centering
        \includegraphics[width=\linewidth]{figures/experiments/balanced_unbalanced_classes.pdf}
        \caption{Your Figure Caption Here}
        \label{fig:balanced_unbalanced_classes}
    \end{figure}
}
\fi

\subsection*{Class Granularity}
We provide multiple label configurations for our dataset designed to address varying levels of class granularity, from fine-grained to coarse-grained classification. In the \textit{C1} configuration, a fine-grained approach is adopted, defining six distinct classes — \textit{cod}, \textit{whiting}, \textit{haddock}, \textit{hake}, \textit{horse mackerel}, and a catch-all category labeled as \textit{other}. A slightly coarser configuration \textit{C2} condenses the classes to four - \textit{cod}, \textit{whiting}, \textit{haddock}, with \textit{hake} and \textit{horse mackerel} added to the \textit{other} category as these species are not true cods. The \textit{C3} configuration represents intermediate coarse level of granularity by categorizing fish into just two groups - \textit{cod-like} (cod, whiting, haddock) and \textit{other}. Lastly, the \textit{C4} configuration simplifies the classification task to a single category \textit{fish}. The label configurations are summed up in Table~\ref{tab:label-configurations}.

This progression across label configurations from fine-grained distinctions to coarser groupings offers adaptability to diverse research objectives, providing researchers with flexibility in choosing the appropriate level of granularity for their specific analysis. These configurations, as outlined in Table \ref{tab:label-configurations}, serve as a foundation for exploring the dataset's diverse characteristics and accommodating a range of classification needs.

\begin{table}[h]
    \centering
    \caption{We provide four different label configurations, from the fine-grained configuration \textit{C1} to the generic fish configuration \textit{C4}.}
    \label{tab:label-configurations}
    \begin{tabular*}{\linewidth}{cc}
        \toprule
        \textbf{Label} & \textbf{Classes} \\
        \midrule
        \rowcolor[HTML]{EFEFEF}C1 & cod, whiting, haddock, hake, horse mackerel, other\\
        C2 & cod, whiting, haddock, other \\
        \rowcolor[HTML]{EFEFEF}C3 & cod-like, other \\
        C4 & fish \\
        \bottomrule
    \end{tabular*}
\end{table}

%Confusion matrcies + precision recall curves 
%\subsection{Insights}
%This section delves into dynamics that shape model performance. We explore the impact of varying training sample sizes on model efficacy and the relationship between data volume and predictive accuracy. Additionally, we investigate the influence of training split balance, comparing models trained on both balanced and unbalanced splits to discern the effects on classification outcomes. Next, the robustness and generalizability are tested as we investigate model's ability to train on images from one camera and test on images from the other camera. These experiments aim to enrich our understanding of model behavior but also contribute practical insights crucial for optimizing performance across diverse scenarios and datasets.
\begin{figure*}
    \centering
    \begin{subfigure}{\textwidth}
        \centering
        \includegraphics[width=\linewidth]{figures/confusion_matrices/C1.pdf}
    \end{subfigure}
    \vspace{\baselineskip} % Vertical space between subfigures
    \begin{subfigure}{\textwidth}
        \centering
        \includegraphics[width=\linewidth]{figures/confusion_matrices/C2.pdf}
    \end{subfigure}
\end{figure*}
\begin{figure*}
    \ContinuedFloat
    \centering
    \begin{subfigure}{\textwidth}
        \centering
        \includegraphics[width=\linewidth]{figures/confusion_matrices/C3.pdf}
    \end{subfigure}
    \vspace{\baselineskip} % Vertical space between subfigures
    \begin{subfigure}{\textwidth}
        \centering
        \includegraphics[width=\linewidth]{figures/confusion_matrices/C4.pdf}
    \end{subfigure}
    \caption{Normalized confusion matrices. Column \textit{bg (FN)} was normalized over the number of instances in the test groups. All other columns were normalized over the column sum.} 
    \label{fig:confusion_matrices}
\end{figure*}

\begin{table}[hbt]
\caption{Overview of the fish groupings with respect to species and number of individuals.}
\label{tab:fish-distribution}
\setlength{\tabcolsep}{2pt}
\begin{tabular*}{\textwidth}{@{\extracolsep{\fill}}lcccccccccccccccccccccccccc@{}}
\toprule
\textbf{Group number}   & 1  & 2  & 3  & 4  & 5  & 6  & 7  & 8  & 9  & 10 & 11 & 12 & 13 & 14 & 15 & 16 & 17 & 18 & 19 & 20 & 21 & 22 & 23 & 24 & 25 & All\\ \midrule
\textbf{Cod}            & 2  & 8  & 4  & 1  & 7  & 1  & 3  & 4  & 3  & 6  & 3  & 4  & 2  & 5  & 8  & 6  & 3  & 1  & 3  & 4  & 6  & 0  & 4  & 2  & 12 & 102\\ 
\textbf{Haddock}        & 4  & 3  & 1  & 4  & 8  & 5  & 4  & 6  & 11 & 8  & 4  & 4  & 5  & 7  & 5  & 2  & 10 & 3  & 4  & 1  & 4  & 5  & 3  & 2  & 6 & 119\\
\textbf{Whiting}        & 5  & 4  & 3  & 5  & 4  & 5  & 2  & 5  & 4  & 2  & 5  & 4  & 7  & 6  & 3  & 5  & 2  & 3  & 6  & 2  & 4  & 7  & 4  & 3  & 3  &  103\\
\textbf{Hake}           & 3  & 1  & 2  & 4  & 1  & 1  & 1  & 3  & 3  & 3  & 2  & 2  & 5  & 0  & 1  & 3  & 2  & 4  & 1  & 2  & 3  & 2  & 0  & 2  & 1 &  52\\
\textbf{Horse mackerel} & 2  & 2  & 2  & 3  & 2  & 3  & 4  & 1  & 2  & 3  & 2  & 1  & 1  & 2  & 2  & 0  & 2  & 3  & 0  & 4  & 0  & 2  & 3  & 3  & 0 & 49\\
\textbf{Other}          & 0  & 1  & 3  & 5  & 0  & 1  & 0  & 1  & 1  & 1  & 0  & 1  & 2  & 1  & 1  & 2  & 1  & 1  & 0  & 3  & 0  & 1  & 0  & 2  & 1 & 29\\ \midrule
\textbf{Total fish}     & 16 & 19 & 15 & 22 & 22 & 16 & 14 & 20 & 24 & 23 & 16 & 16 & 22 & 21 & 20 & 18 & 20 & 15 & 14 & 16 & 17 & 17 & 14 & 14 & 23 & 454 \\ \bottomrule
\end{tabular*}
\end{table}

\begin{figure}
    \centering
    \includegraphics[width=0.7\linewidth]{figures/length_plot.png}
    \caption{Distribution of length measurements of all the fish, conducted by a marine biologists. The lengths are rounded to nearest 5 mm, following common practice.}
    \label{fig:length_compo}
\end{figure}

\lstset{
  basicstyle=\ttfamily\footnotesize,
  stepnumber=1,
  numbersep=5pt,
  backgroundcolor=\color{gray!10},
  frame=single,
  rulecolor=\color{black},
  keywordstyle=\color{blue},
  commentstyle=\bfseries\color{black},
  comment=[l]{\#}, % Set the comment sign to #
  breaklines=true,
  showstringspaces=false,
  captionpos=b,
  morekeywords={Sets, Set1, Set2, set, All},
}

 \begin{lstlisting}[caption={Procedure for acquiring the images of a single group of fish.},label={lst:acquisition}]
 # Initial step
 Assign a unique ID to every fish in the group

 # Split the group with N fish into two sets
 All = [Fish 1, Fish 2, ..., Fish N]
 Set1 = All[:N/2]
 Set2 = All[N/2:]

 # Sets to process
 Sets = [Set1, Set2, All]

 # Image Capture Procedure
 for set in Sets:
     Randomly place fish on the conveyor belt
   
     # Initial side
     Repeat 10 times:
         Capture an image
         Point-annotate every fish with its ID in the image
         Randomly reposition the fish without flipping
   
     # Flipped side
     Flip all fish
     Repeat 10 times:
         Capture an image
         Point-annotate every fish with its ID in the image
         Randomly reposition the fish without flipping
 \end{lstlisting}
